# Supplementary material for: Powerful Design of Small Vision Transformer on CIFAR10
Source: arXiv:2501.06220 source file (2025-01-07)
Supplement: Supplementary file 1 [file X_suppl.tex]

\clearpage
\setcounter{page}{1}
\maketitlesupplementary

\section{Flash attention with compression}

\paragraph{Compile Environment.}
\begin{verbatim}
micromamba install conda-forge::gcc conda-forge::g++  conda-forge::cxx-compiler -y
micromamba install conda-forge::cudatoolkit-dev  nvidia/label/cuda-12.1.1::cuda-toolkit -y
python setup.py install
\end{verbatim}

\paragraph{Entrance}
% https://gordicaleksa.medium.com/eli5-flash-attention-5c44017022ad

https://github.com/tspeterkim/flash-attention-minimal/tree/main?tab=readme-ov-file

\begin{verbatim}
API: https://github.com/Dao-AILab/flash-attention/blob/main/flash_attn/flash_attn_triton.py#L812

https://github.com/Dao-AILab/flash-attention/blob/main/flash_attn/flash_attn_triton.py#L66
\end{verbatim}

\section{Rationale}
\label{sec:rationale}
Having the supplementary compiled together with the main paper means that:
\begin{itemize}
\item The supplementary can back-reference sections of the main paper, for example, we can refer to \cref{sec:intro};
\item The main paper can forward reference sub-sections within the supplementary explicitly (e.g. referring to a particular experiment); 
\item When submitted to arXiv, the supplementary will already included at the end of the paper.
\end{itemize}
To split the supplementary pages from the main paper, you can use \href{https://support.apple.com/en-ca/guide/preview/prvw11793/mac#:~:text=Delete%20a%20page%20from%20a,or%20choose%20Edit%20%3E%20Delete).}{Preview (on macOS)}, \href{https://www.adobe.com/acrobat/how-to/delete-pages-from-pdf.html#:~:text=Choose%20%E2%80%9CTools%E2%80%9D%20%3E%20%E2%80%9COrganize,or%20pages%20from%20the%20file.}{Adobe Acrobat} (on all OSs), as well as \href{https://superuser.com/questions/517986/is-it-possible-to-delete-some-pages-of-a-pdf-document}{command line tools}.
